# Supplementary material for: Linear exciton Hall and Nernst effects in monolayer two-dimensional semiconductors
Source: arXiv:2512.24153 source file (2025-12-30)
Supplement: Supplementary file 1 [file Supp.pdf]

# Supplementary: Linear exciton Hall and Nernst effects in monolayer two-dimensional semiconductors

Weilong Guo,[1] Lianguo Li,[1] Qingjun Tong,[1] and Ci Li[1,*]

[1] *School of Physics and Electronics, Hunan University, Changsha 410082, China*

## S1. General symmetry analysis of non-zero linear exciton Hall current in the monolayer two-dimensional material

### A. Conductivity tensor and symmetry constraints in 2D electronic systems

In a two-dimensional (2D) electronic system, the conductivity $\boldsymbol{\sigma}$ can be expressed as a $2 \times 2$ tensor when only the linear response to an external electric field $\boldsymbol{E} = (E_x, E_y)$ is considered [1, 2]. Ohm's law then takes the form

$$\boldsymbol{j} = \boldsymbol{\sigma}\boldsymbol{E},$$

i.e.,

$$\begin{pmatrix} j_x \\ j_y \end{pmatrix} = \begin{pmatrix} \sigma_{xx} & \sigma_{xy} \\ \sigma_{yx} & \sigma_{yy} \end{pmatrix} \begin{pmatrix} E_x \\ E_y \end{pmatrix},$$

where $\boldsymbol{j} = (j_x, j_y)$ is the 2D electric current density. In the presence of time-reversal ($\mathcal{T}$) symmetry, the conductivity tensor $\boldsymbol{\sigma}$ is associated with dissipative, irreversible processes, because the current density $\boldsymbol{j}$ is $\mathcal{T}$-odd (changes sign under $\mathcal{T}$), while the electric field $\boldsymbol{E}$ is $\mathcal{T}$-even [2, 3]. Moreover, for a system whose microscopic dynamics are governed by a $\mathcal{T}$-symmetric Hamiltonian, the Onsager reciprocal relations impose $\sigma_{xy} = \sigma_{yx}$ [2, 3]. For a nontrivial Hall response under preserved $\mathcal{T}$ symmetry, the off-diagonal conductivity $\sigma_{xy}$ would need to be a nonzero $\mathcal{T}$-odd quantity. This is generally incompatible with time-reversal symmetry in most 2D electronic materials. By contrast, if $\mathcal{T}$ symmetry is broken, $\boldsymbol{\sigma}$ can become $\mathcal{T}$-even and the Onsager relation can be violated, greatly relaxing the symmetry constraints on 2D electronic transport, including Hall-type responses.

* lici@hnu.edu.cn

### B. Extension to exciton transport in 2D systems

A similar analysis applies to exciton transport in 2D systems. Let $\boldsymbol{j} = (j_x, j_y)$ now denote the exciton current density, and consider a uniform in-plane driving field

$$\tilde{\boldsymbol{F}} = \left(\tilde{F}_x, \tilde{F}_y\right) = \left(\tilde{F}\cos\theta, \tilde{F}\sin\theta\right),$$

where $\theta$ is the angle between $\tilde{\boldsymbol{F}}$ and the $x$-axis of the in-plane Cartesian coordinates. The driving field $\tilde{\boldsymbol{F}}$ may represent, for example, a mechanical force $\mathcal{F}$, a spacial gradient of chemical potential $\nabla\mu$, or a spacial gradient of temperature $\nabla T$ in the material. In the linear-response regime, one can write the exciton transport relation in complete analogy with the electronic case:

$$\boldsymbol{j} = \boldsymbol{\sigma}\tilde{\boldsymbol{F}}.$$

Since the exciton current density $\boldsymbol{j}$ remains $\mathcal{T}$-odd whereas $\tilde{\boldsymbol{F}}$ is $\mathcal{T}$-even under $\mathcal{T}$ symmetry, the conductivity tensor $\boldsymbol{\sigma}$ in a $\mathcal{T}$-symmetric 2D excitonic system must satisfy

$$\mathcal{T} : \sigma_{xy} = \sigma_{yx},\ \boldsymbol{\sigma} \text{ is } \mathcal{T}\text{-odd}.$$

Thus, the same symmetry-based constraints that apply to electronic Hall transport also govern the possibility of a Hall-like response in excitonic systems, unless time-reversal symmetry is broken.

### C. Point-group symmetries and constraints on $\boldsymbol{\sigma}$ in 2D

Beyond time-reversal symmetry, 2D systems can possess various point-group symmetries. There are ten crystallographic point groups in 2D, namely

$$C_{n=1,2,3,4,6}, D_{n=1,2,3,4,6}$$

which are generated by mirror and rotational symmetry operations [4] (In 2D, space inversion is equivalent to the two-fold rotation). For simplicity, we ignore combinations of mirror/rotation with translations, which would lead to the 17 wallpaper (space) groups in the 2D plane [4]. The allowed in-plane rotational ($R_\varphi$) and mirror ($M_\phi$) symmetric operations can be written in matrix form as

$$R_\varphi = \begin{pmatrix} \cos\varphi & -\sin\varphi \\ \sin\varphi & \cos\varphi \end{pmatrix}, M_\phi = \begin{pmatrix} \cos 2\phi & \sin 2\phi \\ \sin 2\phi & -\cos 2\phi \end{pmatrix}.$$

Here is the rotation angle for an $n$-fold rotation axis, and $\phi$ is the angle between the in-plane projection of the mirror line and the $x$-axis of the 2D Cartesian coordinate system. These symmetry operations impose additional constraints on the form of the conductivity tensor $\boldsymbol{\sigma}$, further restricting which components (e.g., Hall-type responses) are allowed or forbidden in a given 2D crystal.

*1. Rotational symmetry*

If a 2D material has an $n$-fold rotational symmetry, $\boldsymbol{\sigma}$ must be invariant under the corresponding rotation. Denoting the current and driving field in the rotated frame $\left(j'_x, j'_y\right)$ and $\left(\tilde{F}_x, \tilde{F}_y\right)$, respectively, we have

$$
\begin{aligned}
\begin{pmatrix} j'_x \\ j'_y \end{pmatrix} &= R_\varphi \begin{pmatrix} j_x \\ j_y \end{pmatrix} = R_\varphi \begin{pmatrix} \sigma_{xx} & \sigma_{xy} \\ \sigma_{yx} & \sigma_{yy} \end{pmatrix} R_\varphi^{-1} R_\varphi \begin{pmatrix} \tilde{F}_x \\ \tilde{F}_y \end{pmatrix} \\
&= R_\varphi \begin{pmatrix} \sigma_{xx} & \sigma_{xy} \\ \sigma_{yx} & \sigma_{yy} \end{pmatrix} R_\varphi^{-1} \begin{pmatrix} \tilde{F}'_x \\ \tilde{F}'_y \end{pmatrix} \\
&= \begin{pmatrix} \sigma_{xx} & \sigma_{xy} \\ \sigma_{yx} & \sigma_{yy} \end{pmatrix} \begin{pmatrix} \tilde{F}'_x \\ \tilde{F}'_y \end{pmatrix},
\end{aligned}
$$

Thus, rotational invariance requires $R_\varphi \boldsymbol{\sigma} R_\varphi^{-1} = \boldsymbol{\sigma}$. It is convenient to introduce the following symmetric (S) and antisymmetric (AS) combinations:

$$
\begin{aligned}
\sigma_{\alpha\alpha}^{\mathrm{S}} &= \sigma_{xx} + \sigma_{yy}, \sigma_{\alpha\alpha}^{\mathrm{AS}} = \sigma_{xx} - \sigma_{yy}, \\
\sigma_{\alpha\beta}^{\mathrm{S}} &= \sigma_{xy} + \sigma_{yx}, \sigma_{\alpha\beta}^{\mathrm{AS}} = \sigma_{xy} - \sigma_{yx}.
\end{aligned}
$$

In terms of these, rotational invariance yields

$$
\begin{aligned}
\sigma_{xx} &= \frac{\sigma_{\alpha\alpha}^{\mathrm{S}} + \sigma_{\alpha\alpha}^{\mathrm{AS}} \cos 2\varphi - \sigma_{\alpha\beta}^{\mathrm{AS}} \sin 2\varphi}{2}, \\
\sigma_{xy} &= \frac{\sigma_{\alpha\beta}^{\mathrm{AS}} + \sigma_{\alpha\alpha}^{\mathrm{AS}} \sin 2\varphi + \sigma_{\alpha\beta}^{\mathrm{S}} \cos 2\varphi}{2}, \\
\sigma_{yx} &= \frac{-\sigma_{\alpha\beta}^{\mathrm{AS}} + \sigma_{\alpha\alpha}^{\mathrm{AS}} \sin 2\varphi + \sigma_{\alpha\beta}^{\mathrm{S}} \cos 2\varphi}{2}, \\
\sigma_{yy} &= \frac{\sigma_{\alpha\alpha}^{\mathrm{S}} - \sigma_{\alpha\alpha}^{\mathrm{AS}} \cos 2\varphi + \sigma_{\alpha\beta}^{\mathrm{AS}} \sin 2\varphi}{2},
\end{aligned}
\tag{S1}
$$

### 2. *Mirror symmetry*

Similarly, if the system has a mirror symmetry whose projection in the 2D plane makes an angle $\phi$ with respect to the $x$-axis, invariance of $\boldsymbol{\sigma}$ under the mirror operator $M_\phi$ requires $M_\varphi \boldsymbol{\sigma} M_\varphi^{-1} = \boldsymbol{\sigma}$, i.e.,

$$\begin{pmatrix} \sigma_{xx} & \sigma_{xy} \\ \sigma_{yx} & \sigma_{yy} \end{pmatrix} = M_\phi \begin{pmatrix} \sigma_{xx} & \sigma_{xy} \\ \sigma_{yx} & \sigma_{yy} \end{pmatrix} M_\phi^{-1},$$

which leads to

$$\begin{aligned} \sigma_{xx} &= \frac{\sigma^{\mathrm{S}}_{\alpha\alpha} + \sigma^{\mathrm{AS}}_{\alpha\alpha}\cos 4\phi + \sigma^{\mathrm{S}}_{\alpha\beta}\sin 4\phi}{2}, \\ \sigma_{xy} &= \frac{-\sigma^{\mathrm{AS}}_{\alpha\beta} + \sigma^{\mathrm{AS}}_{\alpha\alpha}\sin 4\phi - \sigma^{\mathrm{S}}_{\alpha\beta}\cos 4\phi}{2}, \\ \sigma_{yx} &= \frac{\sigma^{\mathrm{AS}}_{\alpha\beta} + \sigma^{\mathrm{AS}}_{\alpha\alpha}\sin 4\phi - \sigma^{\mathrm{S}}_{\alpha\beta}\cos 4\phi}{2}, \\ \sigma_{yy} &= \frac{\sigma^{\mathrm{S}}_{\alpha\alpha} - \sigma^{\mathrm{AS}}_{\alpha\alpha}\cos 4\phi - \sigma^{\mathrm{S}}_{\alpha\beta}\sin 4\phi}{2}. \end{aligned} \tag{S2}$$

### 3. *Point-group constraints in 2D*

Neglecting the lowest symmetry groups $C_1$ and $D_1$, which rarely occur in realistic 2D crystals, these symmetry relations imply the following constraints for each 2D point group:

1. $C_2$ ($\varphi = \pi$; no mirror):

no additional constraint on $\boldsymbol{\sigma}$.

2. $C_3$ ($\varphi = 2\pi/3, 4\pi/3$; no mirror):

$\sigma_{yy} = \sigma_{xx}$, $\sigma_{yx} = -\sigma_{xy}$.

3. $C_4$ ($\varphi = \pi/2, \pi, 3\pi/2$; no mirror):

$\sigma_{yy} = \sigma_{xx}$, $\sigma_{yx} = -\sigma_{xy}$.

4. $C_6$ ($\varphi = \pi/3, 2\pi/3, \pi, 4\pi/3, 5\pi/3$; no mirror):

$\sigma_{yy} = \sigma_{xx}$, $\sigma_{yx} = -\sigma_{xy}$.

5. $D_2$ (rhombus/rectangles; $\varphi = \pi$, $\phi = 0, \pi/2$):

$\sigma_{xy} = \sigma_{yx} = 0$.

6. $D_3$ (equilateral triangle; $\varphi = 2\pi/3, 4\pi/3$, $\phi = 0, \pi/3, 2\pi/3$):

$\sigma_{yy} = \sigma_{xx}$, $\sigma_{xy} = \sigma_{yx} = 0$.

7. $D_4$ (square; $\varphi = \pi/2, \pi, 3\pi/2$, $\phi = 0, \pi/4, \pi/2, 3\pi/4$):

$\sigma_{yy} = \sigma_{xx}$, $\sigma_{xy} = \sigma_{yx} = 0$.

8. $D_6$ (hexagonal lattice; $\varphi = \pi/3, 2\pi/3, \pi, 4\pi/3, 5\pi/3$, $\phi = 0, \pi/6, \pi/3, \pi/2, 2\pi/3, 5\pi/6$):

$\sigma_{yy} = \sigma_{xx}$, $\sigma_{xy} = \sigma_{yx} = 0$.

### *4. Conductivity in the field-aligned frame*

It is often convenient to rotate the coordinate system such that the new longitudinal axis $\|$ is aligned with the driving field $\tilde{\boldsymbol{F}} = \left(\tilde{F}_x, \tilde{F}_y\right) = \left(\tilde{F}\cos\theta, \tilde{F}\sin\theta\right)$. In the rotated frame $(\|, \perp)$,

$$\begin{aligned}\begin{pmatrix} j_\| \\ j_\perp \end{pmatrix} &= R_\theta^{-1} \begin{pmatrix} j_x \\ j_y \end{pmatrix} = R_\theta^{-1} \begin{pmatrix} \sigma_{xx} & \sigma_{xy} \\ \sigma_{yx} & \sigma_{yy} \end{pmatrix} R_\theta R_\theta^{-1} \begin{pmatrix} \tilde{F}_x \\ \tilde{F}_y \end{pmatrix} \\ &= R_\theta^{-1} \begin{pmatrix} \sigma_{xx} & \sigma_{xy} \\ \sigma_{yx} & \sigma_{yy} \end{pmatrix} R_\theta \begin{pmatrix} \tilde{F} \\ 0 \end{pmatrix} = \boldsymbol{\sigma'} \begin{pmatrix} \tilde{F} \\ 0 \end{pmatrix},\end{aligned} \tag{S3}$$

where $\boldsymbol{\sigma'} = R_\theta \boldsymbol{\sigma} R_\theta^{-1}$ is the conductivity tensor in the $(\|, \perp)$ frame:

$$\boldsymbol{\sigma'} = \begin{pmatrix} \sigma_\| & \sigma_H^1 \\ \sigma_H^2 & \sigma_\perp \end{pmatrix}.$$

In terms of $\sigma_{\alpha\alpha}^{\mathrm{S,AS}}$ and $\sigma_{\alpha\beta}^{\mathrm{S,AS}}$, we obtain

$$\begin{aligned}\sigma_\| &= \frac{\sigma_{\alpha\alpha}^{\mathrm{S}} + \sigma_{\alpha\alpha}^{\mathrm{AS}}\cos 2\theta + \sigma_{\alpha\beta}^{\mathrm{S}}\sin 2\theta}{2}, \\ \sigma_H^1 &= \frac{\sigma_{\alpha\beta}^{\mathrm{AS}} - \sigma_{\alpha\alpha}^{\mathrm{AS}}\sin 2\theta + \sigma_{\alpha\beta}^{\mathrm{S}}\cos 2\theta}{2}, \\ \sigma_H^2 &= \frac{-\sigma_{\alpha\beta}^{\mathrm{AS}} - \sigma_{\alpha\alpha}^{\mathrm{AS}}\sin 2\theta + \sigma_{\alpha\beta}^{\mathrm{S}}\cos 2\theta}{2}, \\ \sigma_\perp &= \frac{\sigma_{\alpha\alpha}^{\mathrm{S}} - \sigma_{\alpha\alpha}^{\mathrm{AS}}\cos 2\theta - \sigma_{\alpha\beta}^{\mathrm{S}}\sin 2\theta}{2}.\end{aligned} \tag{S4}$$

The key observation is that only the contribution from $\sigma_{\alpha\beta}^{\mathrm{AS}} = \sigma_{xy} - \sigma_{yx}$ to the transverse current is independent of the direction $\theta$ of the driving field. This term corresponds to the conventional Hall response which is non-dissipative [1–3]. Combining $\mathcal{T}$ symmetry with the above point-group constraints, we obtain:

1. $C_2 + \mathcal{T}$:

$\mathcal{T}$ symmetry enforces $\sigma_{xy} = \sigma_{yx} \Longrightarrow \sigma_{\alpha\beta}^{\mathrm{AS}} = 0$. All components of $\boldsymbol{\sigma'}$ can, in principle, be nonzero.

2. $C_{n\geq 3} + \mathcal{T}$:

$\sigma_{yy} = \sigma_{xx}$, $\sigma_{yx} = \sigma_{xy} = 0 \Longrightarrow \sigma^{\mathrm{AS}}_{\alpha\beta} = \sigma^{\mathrm{S}}_{\alpha\beta} = \sigma^{\mathrm{AS}}_{\alpha\alpha} = 0$, and hence $\sigma_{\parallel} = \sigma^{\mathrm{S}}_{\alpha\alpha}/2 = \sigma_{xx} = \sigma_{\perp}$, $\sigma^1_H = \sigma^2_H = 0$.

3. $D_2 + \mathcal{T}$:

$\sigma_{xy} = \sigma_{yx} = 0 \Longrightarrow \sigma^{\mathrm{AS}}_{\alpha\beta} = \sigma^{\mathrm{S}}_{\alpha\beta} = 0$, All components of $\boldsymbol{\sigma}'$ can be nonzero.

4. $D_{n\geq 3} + \mathcal{T}$ : $\sigma_{yy} = \sigma_{xx}$, $\sigma_{yx} = \sigma_{xy} = 0 \Longrightarrow \sigma^{\mathrm{AS}}_{\alpha\beta} = \sigma^{\mathrm{S}}_{\alpha\beta} = \sigma^{\mathrm{AS}}_{\alpha\alpha} = 0$, and $\sigma_{\parallel} = \sigma^{\mathrm{S}}_{\alpha\alpha}/2 = \sigma_{xx} = \sigma_{\perp}$, $\sigma^1_H = \sigma^2_H = 0$.

Since monolayer transition metal dichalcogenides (TMDs) possess $D_{3h}$ point-group symmetry [5, 6] and monolayer black phosphorus (BP) possesses $D_{2h}$ symmetry [8, 9], they fall into cases 4 and 3, respectively, in the above classification. The corresponding symmetry-imposed constraints on the exciton current conductivity tensor are summarized in Table I of the main text.

## D. Momentum-space symmetry and conditions for linear exciton Hall response

From the momentum-space perspective—particularly the symmetry of effective band-edge Hamiltonians near high-symmetry points in the first Brillouin zone—it is clear that a nonzero *linear* exciton Hall current in a monolayer 2D material requires a finite exciton Berry curvature $\Omega^{ex} \neq 0$. In the band-edge model considered here, this condition can be written as

$$\frac{m_{e,x}m_{e,y}}{m_{ex,x}m_{ex,y}}\Omega_c - \frac{m_{h,x}m_{h,y}}{m_{ex,x}m_{ex,y}}\Omega_v \neq 0,$$

or $2\theta \neq n\pi\,(n \in Z)$ with $\sigma^1_{xx} \neq \sigma^1_{yy}\left(\alpha^1_{xx} \neq \alpha^1_{yy}\right)$. The first condition can be self-satisfied when there is non-zero $\Omega_{c(v)}$ that comes from the broken of $\mathcal{T}$ or spacial inversion ($\mathcal{S}$) symmetry in the effective electric band-edge model due to $\Omega_c = -\Omega_v$. In a generic two-band band-edge model [Eq. (9) in the main text] with crystal momentum $\boldsymbol{Q} = (Q_x, Q_y)$

$$\begin{aligned} H^e &= \begin{pmatrix} \varepsilon_g/2 + \eta_c Q_x^2 + \nu_c Q_y^2 & c_1 Q_x - i c_2 Q_y \\ c_1 Q_x + i c_2 Q_y & -\varepsilon_g/2 + \eta_v Q_x^2 + \nu_v Q_y^2 \end{pmatrix} \\ &= \frac{C}{2} + \frac{1}{2}\begin{pmatrix} A & Be^{-i\varphi} \\ Be^{i\varphi} & -A \end{pmatrix}, \end{aligned} \tag{S5}$$

which is a good approximation for many monolayer 2D materials. Here

$$A=\Delta+\left(\eta_c-\eta_v\right)Q_x^2+\left(v_c-v_v\right)Q_y^2, B=2\sqrt{c_1^2Q_x^2+c_2^2Q_y^2},$$
$$C=\left(\eta_c+\eta_v\right)Q_x^2+\left(v_c+v_v\right)Q_y^2, \varphi=\arctan\left(c_2Q_y/c_1Q_x\right),$$

$i$ is the imaginary unit, $\Delta=\varepsilon_g$ is the band gap, and all other parameters are real number. If all parameters are non-zero, one finds the generalized relation (for the effective electric band-edge model such as *valley Hamiltonians*) $H^e\left(\boldsymbol{Q}\right)=\sigma_z H^e\left(-\boldsymbol{Q}\right)\sigma_z$, while $\mathcal{T}$ can be effectively broken. The Berry curvature of the conduction ($c$) and valence ($v$) bands,

$$\begin{aligned}\Omega_c\left(\boldsymbol{Q}\right)&=\nabla_{\boldsymbol{Q}}\times i\left\langle c\right|\partial_{\boldsymbol{Q}}\left|c\right\rangle=i\left(\mathcal{R}_{cv}^x\mathcal{R}_{vc}^y-\mathcal{R}_{cv}^y\mathcal{R}_{vc}^x\right)\\&=-2\mathrm{Im}\mathcal{R}_{cv}^x\mathcal{R}_{vc}^y=-\Omega_v\left(\boldsymbol{Q}\right)\\&=\frac{c_1c_2\left[2\left(\eta_c-\eta_v\right)Q_x^2+2\left(v_c-v_v\right)Q_y^2+A\right]}{\left(B^2+A^2\right)^{3/2}},\end{aligned}$$

with $\mathcal{R}_{cv}^{\gamma=x,y}=i\left\langle c\right|\partial_{Q_\gamma}\left|v\right\rangle$ the interband Berry connection. Thus, non-zero $c_1$ and $c_2$ are required to generate $\Omega_c=-\Omega_v\neq0$. The exciton Berry curvature $\Omega^{ex}$ can then be obtained by replacing the electron crystal momentum $\boldsymbol{Q}$ with the exciton center-of-mass momentum $\boldsymbol{k}$.

However, even if $\Omega^{ex}\neq0$ locally (e.g., near each valley), the crystal symmetry of the full Brillouin zone—especially when summing contributions from symmetry-related high-symmetry points such as $\pm K$ in monolayer TMDs—can enforce a net cancellation of Berry curvature, as shown below. In such cases, the global symmetry of the crystal (rather than the symmetry of a single valley Hamiltonian) prevents a net linear exciton Hall (Nernst) effect, consistent with the real-space symmetry analysis presented above.

## S2. Calculation of exciton Berry curvature in monolayer TMDs

According to the effective exciton Hamiltonian $H_{\rm TMD}$ [Eq. (10)] and the related eigenstate [Eq. (11)] in the main text, one can easily find that

$$\begin{aligned}
\mathcal{A}^{ex}_{k_x,L} &= i\left\langle \boldsymbol{k}\right|_L \partial_{k_x}\left|\boldsymbol{k}\right\rangle_L \\
&= i\frac{2i}{2}\frac{-\frac{k_y}{k_x^2}}{1+\left(\frac{k_y}{k_x}\right)^2} + \frac{\sum_{\eta=\pm} i\left\langle \boldsymbol{k}\right|_{\eta K}\partial_{k_x}\left|\boldsymbol{k}\right\rangle_{\eta K}}{2} \\
&= \frac{k_y}{k^2} + \frac{\sum_{\eta=\pm} i\left\langle \boldsymbol{k}\right|_{\eta K}\partial_{k_x}\left|\boldsymbol{k}\right\rangle_{\eta K}}{2}, \\
\mathcal{A}^{ex}_{k_y,L} &= -\frac{k_x}{k^2} + \frac{\sum_{\eta=\pm} i\left\langle \boldsymbol{k}\right|_{\eta K}\partial_{k_y}\left|\boldsymbol{k}\right\rangle_{\eta K}}{2},
\end{aligned}$$

and

$$\begin{aligned}
\Omega_L &= \partial_{k_x}\mathcal{A}^{ex}_{k_y,L} - \partial_{k_y}\mathcal{A}^{ex}_{k_x,L} \\
&= -\frac{1}{k^2} + \frac{2k_x^2}{k^4} - \frac{1}{k^2} + \frac{2k_y^2}{k^4} + \frac{\Omega^{ex}_K + \Omega^{ex}_{-K}}{2} \\
&= \frac{\Omega^{ex}_K + \Omega^{ex}_{-K}}{2}.
\end{aligned} \tag{S6}$$

The similar process tells us that $\Omega_T = \frac{\Omega^{ex}_K+\Omega^{ex}_{-K}}{2}$ with

$$\begin{aligned}
\Omega^{ex}_{\pm K} &\approx \left[\left(\frac{m_e}{m_{ex}}\right)^2\Omega_{\pm K,e} + \left(\frac{m_h}{m_{ex}}\right)^2\Omega_{\pm K,h}\right]\sum_{\boldsymbol{q}}\left|F\right|^2 \\
&= \left[\left(\frac{m_e}{m_{ex}}\right)^2\Omega_{\pm K,c} - \left(\frac{m_h}{m_{ex}}\right)^2\Omega_{\pm K,v}\right]A_s\sum_{\boldsymbol{q}}\frac{\left|F\right|^2}{A_s} \\
&\approx \left(\frac{m_e}{m_{ex}}\right)^2\left[\Omega_{\pm K,c} - \Omega_{\pm K,v}\right]\frac{A_s}{a_B^2},
\end{aligned}$$

$A_s = \sqrt{3}a^2$ ($a \approx 3.31\,$Å is the lattice constant) is the area of the unit cell. $a_B \approx 1\,$nm is the exciton Bohr radius for monolayer TMDs, where $\sum_{\boldsymbol{q}}\frac{|F|^2}{A} \approx 1/a_B^2$ since the real space wavefunction for the relative motion between electron and hole can be approximately solved by the Schrodinger equation of the hydrogen-like atom [10]. The effective electric band-edge model $H^e_{\rm TMD}$ fitted from the first-principle calculations has a form as [5, 6]

$$H^e_{\rm TMD} \simeq \frac{\tau s_z\lambda}{2} + \begin{bmatrix} \left(\Delta - \tau s_z\lambda\right)/2 & at\left(\tau Q_x - iQ_y\right) \\ at\left(\tau Q_x + iQ_y\right) & -\left(\Delta - \tau s_z\lambda\right)/2 \end{bmatrix}. \tag{S7}$$

The effective hopping integral $t \approx 1.19\,$eV, and the energy gap $\Delta \approx 2.73\,$eV. $\tau = \pm 1$ is the valley index. $s_z = \pm 1$ is the spin index [spin up (↑) for $+1$ and spin down (↓) for $-1$]. $2\lambda \approx$

0.46 eV is the spin splitting at the valence band top caused by the spin-orbit coupling. Here the energy gap $\Delta$ has been corrected by the data from GW calculations [7, 11–14] to avoid underestimating the electronic band gap due to density function theory calculations. By taking $A = \Delta - \tau s_z \lambda$, $B = at\tau|\boldsymbol{Q}|$, $c_1 = at\tau$, and $c_2 = at$ based on the Eq. (9) in main text, it is obvious that $\sigma_x \left[H^e_{\mathrm{TMD}}(\boldsymbol{Q})\right]^* \sigma_x = -H^e_{\mathrm{TMD}}(-\boldsymbol{Q})$ and $\sigma_z H^e_{\mathrm{TMD}}(\boldsymbol{Q}) \sigma_z = H^e_{\mathrm{TMD}}(-\boldsymbol{Q})$, which means $\mathcal{C}$ and $\mathcal{S}$ symmetries are preserved but broken $\mathcal{T}$ symmetry, resulting in non-zero

$$\Omega_c(\boldsymbol{Q}) = \frac{-2a^2t^2\tau A}{\left(B^2 + A^2\right)^{3/2}} = -\Omega_v(\boldsymbol{Q}). \tag{S8}$$

## S3. Calculation of linear exciton Hall/Nernst effect

As we illustrated in the main text, from previous theoretical works [15–17], the current density of excitons in the intrinsic response can be expressed as

$$\begin{aligned} \boldsymbol{j} &= \boldsymbol{j}_0 + \boldsymbol{j}_1, \\ \boldsymbol{j}_0 &= \sum_n \int \left[\frac{d^2\boldsymbol{k}}{(2\pi)^2} f_n^0(\boldsymbol{k})\, \boldsymbol{v}_n(\boldsymbol{k}) + \nabla \times \boldsymbol{M}(r)\right], \\ \boldsymbol{j}_1 &= \sum_n \int \frac{d^2\boldsymbol{k}}{(2\pi)^2} f_n^1(\boldsymbol{k})\, \boldsymbol{v}_n(\boldsymbol{k}), \end{aligned} \tag{S9}$$

where $n$ is the band index for different excitonic bands.

$$\boldsymbol{v}_n(\boldsymbol{k}) = \frac{\partial \varepsilon_n(\boldsymbol{k})}{\hbar \partial \boldsymbol{k}} - \frac{\boldsymbol{\mathcal{F}}}{\hbar} \times \Omega_{n,\boldsymbol{k}} \hat{z} = \boldsymbol{v}_b + \boldsymbol{v}_a,$$

is the velocity of an exciton. $\boldsymbol{v}_b \equiv \frac{\partial \varepsilon_n(\boldsymbol{k})}{\hbar \partial \boldsymbol{k}}$ means the band velocity, which is similar with the one for electronic systems. $\boldsymbol{\mathcal{F}} = \hbar \frac{d\boldsymbol{k}}{dt}$ represents the in-plane driving force.

$$\boldsymbol{M}(r) = \frac{k_B T}{\hbar} \sum_n \int \frac{d^2\boldsymbol{k}}{(2\pi)^2} \Omega_{n,\boldsymbol{k}} \hat{z} \log\left[1 - e^{-(\varepsilon_n - \mu)/k_B T}\right],$$

is analogous to the equilibrium magnetization density in electronic systems [15, 16]. Here $f_n^0(\boldsymbol{k}) = 1/\left[e^{(\varepsilon_n - \mu)/k_B T} - 1\right]$ is the equilibrium Bose-Einstein distribution function and $f_n^1(\boldsymbol{k}) = -\tau d f_n^0(\boldsymbol{k})/dt$. $\boldsymbol{j}_1$ comes from the general expansion of electric direct current (DC) density based on the Boltzmann equation [18], which can be explicitly expressed as

$$\begin{aligned} \boldsymbol{j}_1 &= \sum_n \int \frac{d^2\boldsymbol{k}}{(2\pi)^2} f_n^1(\boldsymbol{k})\, \boldsymbol{v}_n(\boldsymbol{k}) \\ &= -\sum_n \int \tau(\boldsymbol{k}) \frac{d^2\boldsymbol{k}}{(2\pi)^2} \left[\dot{\boldsymbol{x}}_n \cdot \nabla f_n^0(\boldsymbol{k}) + \hbar \dot{\boldsymbol{k}} \cdot \nabla_{\hbar \boldsymbol{k}} f_n^0(\boldsymbol{k}) + \partial_t f_n^0(\boldsymbol{k})\right] \boldsymbol{v}_n(\boldsymbol{k}). \end{aligned}$$

Normally, $f_n^0(\boldsymbol{k})$ is independent with the spatial coordinate $\boldsymbol{x}$ and not explicitly with respect to time $t$, i.e., $\nabla f_n^0(\boldsymbol{k}) = 0$, $\partial_t f_n^0(\boldsymbol{k}) = 0$. In our consideration, we suppose that there is a spacial distribution for the chemical potential $\mu$ and temperature $T$, i.e., $\nabla\mu$ $(\nabla T) \neq 0$, and take a general assumption that the relaxation time $\tau(\boldsymbol{k}) \equiv \tau$ is a constant, leading to

$$
\begin{aligned}
\boldsymbol{j}_1 &= \sum_n \int \frac{d^2\boldsymbol{k}}{(2\pi)^2} f_n^1(\boldsymbol{k})\, \boldsymbol{v}_n(\boldsymbol{k}) \\
&= -\tau \sum_n \int \frac{d^2\boldsymbol{k}}{(2\pi)^2} \left[\dot{\boldsymbol{x}}_n \cdot \nabla f_n^0(\boldsymbol{k}) + \hbar\dot{\boldsymbol{k}} \cdot \nabla_{\hbar\boldsymbol{k}} f_n^0(\boldsymbol{k})\right] \boldsymbol{v}_n(\boldsymbol{k}) \\
&= -\tau \sum_n \int \frac{d^2\boldsymbol{k}}{(2\pi)^2} \{\boldsymbol{v}_n(\boldsymbol{k}) \cdot \left[\partial_\mu f_n^0(\boldsymbol{k})\, \nabla\mu + \partial_T f_n^0(\boldsymbol{k})\, \nabla T\right] \\
&\quad + \boldsymbol{\mathcal{F}} \cdot \frac{\partial\varepsilon_n(\boldsymbol{k})}{\hbar\partial\boldsymbol{k}} \partial_{\varepsilon_n} f_n^0(\boldsymbol{k})\} \boldsymbol{v}_n(\boldsymbol{k}) \\
&\approx -\tau \sum_n \int \frac{d^2\boldsymbol{k}}{(2\pi)^2} \{\frac{\partial\varepsilon_n(\boldsymbol{k})}{\hbar\partial\boldsymbol{k}} \cdot \left[\partial_\mu f_n^0(\boldsymbol{k})\, \nabla\mu + \partial_T f_n^0(\boldsymbol{k})\, \nabla T\right] \\
&\quad + \boldsymbol{\mathcal{F}} \cdot \frac{\partial\varepsilon_n(\boldsymbol{k})}{\hbar\partial\boldsymbol{k}} \partial_{\varepsilon_n} f_n^0(\boldsymbol{k})\} \frac{\partial\varepsilon_n(\boldsymbol{k})}{\hbar\partial\boldsymbol{k}} + O\left(F^2\right),
\end{aligned}
$$

where we have dropped the higher order term of $\boldsymbol{\mathcal{F}}$ or the combination of $\boldsymbol{\mathcal{F}}$, $\nabla T$ and $\nabla\mu$ in the last step since we only focus on the linear transport effect. In 2D systems, the $\mathcal{T}$ symmetry or $\mathcal{S}$ symmetry preserves that $\varepsilon_n(\boldsymbol{k}) = \varepsilon_n(-\boldsymbol{k})$, resulting in $\frac{\partial\varepsilon_n(\boldsymbol{k})}{\hbar\partial\boldsymbol{k}} = \frac{\partial\varepsilon_n(-\boldsymbol{k})}{\hbar\partial\boldsymbol{k}} = -\frac{\partial\varepsilon_n(-\boldsymbol{k})}{\hbar\partial(-\boldsymbol{k})}$. Therefore, only the term as $\left[\frac{\partial\varepsilon_n(\boldsymbol{k})}{\hbar\partial k_\alpha}\right]^2$ can survive in the above integral since it is the even function of $\boldsymbol{k}$, this gives

$$
\boldsymbol{j}_1 \approx \begin{pmatrix} \sigma_{xx}^1 & 0 \\ 0 & \sigma_{yy}^1 \end{pmatrix} \begin{pmatrix} \mathcal{F}_x - \partial_x\mu \\ \mathcal{F}_y - \partial_y\mu \end{pmatrix} - \begin{pmatrix} \alpha_{xx}^1 & 0 \\ 0 & \alpha_{yy}^1 \end{pmatrix} \begin{pmatrix} k_B\partial_x T \\ k_B\partial_y T \end{pmatrix}, \tag{S10}
$$

with

$$\sigma_{\gamma\gamma}^{1} = -\tau\sum_{n}\int\frac{d^{2}\boldsymbol{k}}{\left(2\pi\right)^{2}}\left[\frac{\partial\varepsilon_{n}\left(\boldsymbol{k}\right)}{\hbar\partial k_{\gamma}}\right]^{2}\partial_{\varepsilon_{n}}f_{n}^{0}\left(\boldsymbol{k}\right), \gamma = x, y \tag{S11}$$

$$= \frac{\tau}{k_{B}T}\sum_{n}\int\frac{d^{2}\boldsymbol{k}}{\left(2\pi\right)^{2}}\left[\frac{\partial\varepsilon_{n}\left(\boldsymbol{k}\right)}{\hbar\partial k_{\gamma}}\right]^{2}\frac{e^{\left(\varepsilon_{n}-\mu\right)/k_{B}T}}{\left[e^{\left(\varepsilon_{n}-\mu\right)/k_{B}T}-1\right]^{2}}$$

$$= \frac{\tau}{k_{B}T}\sum_{n}\int\frac{d^{2}\boldsymbol{k}}{\left(2\pi\right)^{2}}v_{b,\gamma}^{2}\left\{f_{n}^{0}\left(\boldsymbol{k}\right)+\left[f_{n}^{0}\left(\boldsymbol{k}\right)\right]^{2}\right\},$$

$$\alpha_{\gamma\gamma}^{1} = \frac{\tau}{k_{B}}\sum_{n}\int\frac{d^{2}\boldsymbol{k}}{\left(2\pi\right)^{2}}\left[\frac{\partial\varepsilon_{n}\left(\boldsymbol{k}\right)}{\hbar\partial k_{\gamma}}\right]^{2}\partial_{T}f_{n}^{0}\left(\boldsymbol{k}\right)$$

$$= \frac{\tau}{k_{B}T^{2}}\sum_{n}\int\frac{d^{2}\boldsymbol{k}}{\left(2\pi\right)^{2}}\left[\frac{\partial\varepsilon_{n}\left(\boldsymbol{k}\right)}{\hbar\partial k_{\gamma}}\right]^{2}\frac{\left(\varepsilon_{n}-\mu\right)e^{\left(\varepsilon_{n}-\mu\right)/k_{B}T}}{k_{B}\left[e^{\left(\varepsilon_{n}-\mu\right)/k_{B}T}-1\right]^{2}}$$

$$= \frac{\tau}{k_{B}T}\sum_{n}\int\frac{d^{2}\boldsymbol{k}}{\left(2\pi\right)^{2}}v_{b,\gamma}^{2}\frac{\varepsilon_{n}-\mu}{k_{B}T}\left\{f_{n}^{0}\left(\boldsymbol{k}\right)+\left[f_{n}^{0}\left(\boldsymbol{k}\right)\right]^{2}\right\}.$$

Then back to $\boldsymbol{j}_0$, the similar analysis for the integral is still effective, giving

$$\boldsymbol{j}_{0} = \sum_{n}\int\frac{d^{2}\boldsymbol{k}}{\left(2\pi\right)^{2}}f_{n}^{0}\left(\boldsymbol{k}\right)\boldsymbol{v}_{n}\left(\boldsymbol{k}\right)+\nabla\times\boldsymbol{M}\left(r\right)$$

$$= -\sum_{n}\int\frac{d^{2}\boldsymbol{k}}{\left(2\pi\right)^{2}}f_{n}^{0}\left(\boldsymbol{k}\right)\left(\frac{\boldsymbol{\mathcal{F}}}{\hbar}\times\Omega_{n,\boldsymbol{k}}\hat{z}\right)+\nabla\mu\times\partial_{\mu}\boldsymbol{M}\left(r\right)+\nabla T\times\partial_{T}\boldsymbol{M}\left(r\right),$$

with

$$\nabla\mu\times\partial_{\mu}\boldsymbol{M}\left(r\right) = -\frac{k_{B}T}{\hbar}\frac{1}{k_{B}T}\sum_{n}\int\frac{d^{2}\boldsymbol{k}}{\left(2\pi\right)^{2}}\left(\nabla_{\mu}\times\Omega_{n,\boldsymbol{k}}\hat{z}\right)\frac{e^{-\left(\varepsilon_{n}-\mu\right)/k_{B}T}}{1-e^{-\left(\varepsilon_{n}-\mu\right)/k_{B}T}}$$

$$= -\frac{1}{\hbar}\sum_{n}\int\frac{d^{2}\boldsymbol{k}}{\left(2\pi\right)^{2}}f_{n}^{0}\left(\boldsymbol{k}\right)\left(\nabla_{\mu}\times\Omega_{n,\boldsymbol{k}}\hat{z}\right),$$

$$\nabla T\times\partial_{T}\boldsymbol{M}\left(r\right) = \frac{k_{B}}{\hbar}\sum_{n}\int\frac{d^{2}\boldsymbol{k}}{\left(2\pi\right)^{2}}\left(\nabla_{T}\times\Omega_{n,\boldsymbol{k}}\hat{z}\right)\log\left[1-e^{-\left(\varepsilon_{n}-\mu\right)/k_{B}T}\right]$$

$$-\frac{k_{B}T}{\hbar}\frac{1}{k_{B}T^{2}}\sum_{n}\int\frac{d^{2}\boldsymbol{k}}{\left(2\pi\right)^{2}}\left(\nabla_{T}\times\Omega_{n,\boldsymbol{k}}\hat{z}\right)\frac{\left(\varepsilon_{n}-\mu\right)e^{-\left(\varepsilon_{n}-\mu\right)/k_{B}T}}{1-e^{-\left(\varepsilon_{n}-\mu\right)/k_{B}T}}$$

$$= \frac{k_{B}}{\hbar T}\sum_{n}\int\frac{d^{2}\boldsymbol{k}}{\left(2\pi\right)^{2}}\left(\nabla_{T}\times\Omega_{n,\boldsymbol{k}}\hat{z}\right)\{T\log\left[1-e^{-\left(\varepsilon_{n}-\mu\right)/k_{B}T}\right]-$$

$$\frac{\varepsilon_{n}-\mu}{k_{B}}f_{n}^{0}\left(\boldsymbol{k}\right)\}.$$

This leads to

$$\boldsymbol{j}_{0} = \begin{pmatrix} 0 & \sigma_{xy}^{0} \\ \sigma_{yx}^{0} & 0 \end{pmatrix}\begin{pmatrix} \mathcal{F}_{x}+\partial_{x}\mu \\ \mathcal{F}_{y}+\partial_{y}\mu \end{pmatrix} - \tag{S12}$$

$$\begin{pmatrix} 0 & \alpha_{xy}^{0} \\ \alpha_{yx}^{0} & 0 \end{pmatrix}\begin{pmatrix} k_{B}\partial_{x}T \\ k_{B}\partial_{y}T \end{pmatrix},$$

with

$$\sigma^0_{xy} = -\frac{1}{\hbar}\sum_n \int \frac{d^2\boldsymbol{k}}{(2\pi)^2} f^0_n(\boldsymbol{k})\,\Omega_{n,\boldsymbol{k}} = -\sigma^0_{xy},$$

$$\begin{aligned}\alpha^0_{xy} &= \frac{1}{\hbar T}\sum_n \int \frac{d^2\boldsymbol{k}}{(2\pi)^2}\Omega_{n,\boldsymbol{k}}\{\frac{\varepsilon_n-\mu}{k_B}f^0_n(\boldsymbol{k}) \\ &\quad -T\log\left[1-e^{-(\varepsilon_n-\mu)/k_BT}\right]\} \\ &= -\alpha^0_{xy}. \end{aligned} \tag{S13}$$

Finally, assume that in-plane driving force $\boldsymbol{\mathcal{F}}$, spacial gradient of chemical potential $\nabla\mu$, and spacial gradient of temperature $\nabla T$ in the same direction for simplicity. According to the analysis in section S1 and Eq. (S4), one can easily derive

$$\begin{aligned}\tilde{\boldsymbol{j}}_0 = R^{-1}_\theta \boldsymbol{j}_0 &= R^{-1}_\theta \begin{pmatrix} 0 & \sigma^0_{xy} \\ \sigma^0_{yx} & 0 \end{pmatrix} R_\theta R^{-1}_\theta \begin{pmatrix} \mathcal{F}_x+\partial_x\mu \\ \mathcal{F}_y+\partial_y\mu \end{pmatrix} \\ &\quad -R^{-1}_\theta \begin{pmatrix} 0 & \alpha^0_{xy} \\ \alpha^0_{yx} & 0 \end{pmatrix} R_\theta R^{-1}_\theta \begin{pmatrix} k_B\partial_x T \\ k_B\partial_y T \end{pmatrix} \\ &= \begin{pmatrix} 0 & \sigma^0_{xy} \\ \sigma^0_{yx} & 0 \end{pmatrix} \begin{pmatrix} \mathcal{F}_\parallel+\partial_\parallel\mu \\ \mathcal{F}_\perp+\partial_\perp\mu \end{pmatrix} \\ &\quad - \begin{pmatrix} 0 & \alpha^0_{xy} \\ \alpha^0_{yx} & 0 \end{pmatrix} \begin{pmatrix} k_B\partial_\parallel T \\ k_B\partial_\perp T \end{pmatrix}, \end{aligned}$$

$$\begin{aligned}\tilde{\boldsymbol{j}}_1 = R^{-1}_\theta \boldsymbol{j}_1 &\approx R^{-1}_\theta \begin{pmatrix} \sigma^1_{xx} & 0 \\ 0 & \sigma^1_{yy} \end{pmatrix} R_\theta R^{-1}_\theta \begin{pmatrix} \mathcal{F}_x-\partial_x\mu \\ \mathcal{F}_y-\partial_y\mu \end{pmatrix} \\ &\quad -R^{-1}_\theta \begin{pmatrix} \alpha^1_{xx} & 0 \\ 0 & \alpha^1_{yy} \end{pmatrix} R_\theta R^{-1}_\theta \begin{pmatrix} k_B\partial_x T \\ k_B\partial_y T \end{pmatrix} \\ &= \begin{pmatrix} \cos^2\theta\sigma^1_{xx}+\sin^2\theta\sigma^1_{yy} & \frac{\sin 2\theta}{2}\left(\sigma^1_{xx}-\sigma^1_{yy}\right) \\ \frac{\sin 2\theta}{2}\left(\sigma^1_{xx}-\sigma^1_{yy}\right) & \sin^2\theta\sigma^1_{xx}+\cos^2\theta\sigma^1_{yy} \end{pmatrix} \begin{pmatrix} \mathcal{F}_\parallel-\partial_\parallel\mu \\ \mathcal{F}_\perp-\partial_\perp\mu \end{pmatrix} \\ &\quad - \begin{pmatrix} \cos^2\theta\alpha^1_{xx}+\sin^2\theta\alpha^1_{yy} & \frac{\sin 2\theta}{2}\left(\alpha^1_{xx}-\alpha^1_{yy}\right) \\ \frac{\sin 2\theta}{2}\left(\alpha^1_{xx}-\alpha^1_{yy}\right) & \sin^2\theta\alpha^1_{xx}+\cos^2\theta\alpha^1_{yy} \end{pmatrix} \begin{pmatrix} k_B\partial_\parallel T \\ k_B\partial_\perp T \end{pmatrix}. \end{aligned} \tag{S14}$$

So the linear exciton Hall current can be expressed as

$$
\begin{aligned}
j_{\|,H} = & \left[\sigma_{xy}^0 + \frac{\sin 2\theta}{2}\left(\sigma_{xx}^1 - \sigma_{yy}^1\right)\right]\mathcal{F}_\perp + \left[\sigma_{xy}^0 - \frac{\sin 2\theta}{2}\left(\sigma_{xx}^1 - \sigma_{yy}^1\right)\right]\partial_\perp \mu \\
& + \left[\alpha_{xy}^0 + \frac{\sin 2\theta}{2}\left(\alpha_{xx}^1 - \alpha_{yy}^1\right)\right]\left(-k_B \partial_\perp T\right), \\
j_{\perp,H} = & \left[\sigma_{yx}^0 + \frac{\sin 2\theta}{2}\left(\sigma_{xx}^1 - \sigma_{yy}^1\right)\right]\mathcal{F}_\| + \left[\sigma_{yx}^0 - \frac{\sin 2\theta}{2}\left(\sigma_{xx}^1 - \sigma_{yy}^1\right)\right]\partial_\| \mu \\
& + \left[\alpha_{yx}^0 + \frac{\sin 2\theta}{2}\left(\alpha_{xx}^1 - \alpha_{yy}^1\right)\right]\left(-k_B \partial_\| T\right). \qquad \text{(S15)}
\end{aligned}
$$

Since $\mathcal{F}_\perp$, $\partial_\perp \mu$ and $\partial_\perp T$ all equals to zero based on the assumption, thus we only have the non-zero $j_{\perp,H}$ in our consideration.

---


[1] D. Xiao, M.-C. Chang, and Q. Niu, Berry phase effects on electronic properties. Rev. Mod. Phys. **82**, 1959 (2010).

[2] Naoto Nagaosa, Jairo Sinova, Shigeki Onoda, A. H. MacDonald, and N. P. Ong, Anomalous Hall effect. Rev. Mod. Phys. **82**, 1539-1592 (2010).

[3] L. D. Landau, E. M. Lifshitz, and L. P. Pitaevskii, *Electrodynamics of Continuous Media, 2nd ed.* (Elsevier, Oxford, 2008).

[4] H. S. M. Coxeter and W. O. J. Moser, *Generators and Relations for Discrete Groups, 4th ed.* (Springer Berlin, Heidelberg, 1980).

[5] Di Xiao, Gui-Bin Liu, Wanxiang Feng, Xiaodong Xu, and Wang Yao, Coupled Spin and Valley Physics in Monolayers of MoS2 and Other Group-VI Dichalcogenides. Phys. Rev. Lett. **108**, 196802 (2012).

[6] Gui-Bin Liu, Wen-Yu Shan, Yugui Yao, Wang Yao, and Di Xiao, Three-band tight-binding model for monolayers of group-VIB transition metal dichalcogenides. Phys. Rev. B **88**, 085433 (2013).

[7] Diana Y. Qiu, Felipe H. da Jornada, and Steven G. Louie, Optical Spectrum of $MoS_2$: Many-Body Effects and Diversity of Exciton States. Phys. Rev. Lett. **111**, 216805 (2013).

[8] A. S. Rodin, A. Carvalho, and A. H. Castro Neto, Strain-Induced Gap Modification in Black Phosphorus. Phys. Rev. Lett. **112**, 176801 (2014).

[9] Pengke Li and Ian Appelbaum, Electrons and holes in phosphorene. Phys. Rev. B **90**, 115439 (2014).

[10] J. Z. Zhang and J. Z. Ma, Two-dimensional excitons in monolayer transition metal dichalcogenides from radial equation and variational calculations. J. Phys.: Condens. Matter **31**, 105702 (2019).

[11] Hongliang Shi, Hui Pan, Yong-Wei Zhang, and Boris I. Yakobson, Quasiparticle band structures and optical properties of strained monolayer $MoS_2$ and $WS_2$. Phys. Rev. B **87**, 155304 (2013).

[12] Diana Y. Qiu, Ting Cao, and Steven G. Louie, Nonanalyticity, Valley quantum phases, and lightlike exciton dispersion in monolayer transition metal dichalcogenides: theory and first-principles calculations. Phys. Rev. Lett. **115**, 176801 (2015).

[13] Kai Hao, et al, Direct measurement of exciton valley coherence in monolayer $WSe_2$. Nat. Phys. **12**, 677-682 (2016).

[14] Nourdine Zibouche, Martin Schlipf, and Feliciano Giustino, GW band structure of monolayer $MoS_2$ using the SternheimerGW method and effect of dielectric environment. Phys. Rev. B **103**, 125401 (2021).

[15] W. Yao and Q. Niu, Berry Phase Effect on the Exciton Transport and on the Exciton Bose-Einstein Condensate. Phys. Rev. Lett. **101**, 106401 (2008).

[16] Di Xiao, Yugui Yao, Zhong Fang, and Qian Niu, Berry-Phase Effect in Anomalous Thermoelectric Transport. Phys. Rev. Lett. **97**, 026603 (2006).

[17] Cong Chen, Dawei Zhai, Cong Xiao, and Wang Yao, Crossed Nonlinear Dynamical Hall Effect in Twisted Bilayer. Phys. Rev. Res **6**, L012059 (2024).

[18] N. W. Ashcroft and N. D. Mermin, *Solid state physics.* (Beijing World Publishing Corporation, 1976) pp. 250, Eq. 13.25.
